# Supplementary material for: Unsupervised Degradation Representation Learning for Blind Super-Resolution
Source: arXiv:2104.00416 source file (2021-04-01)

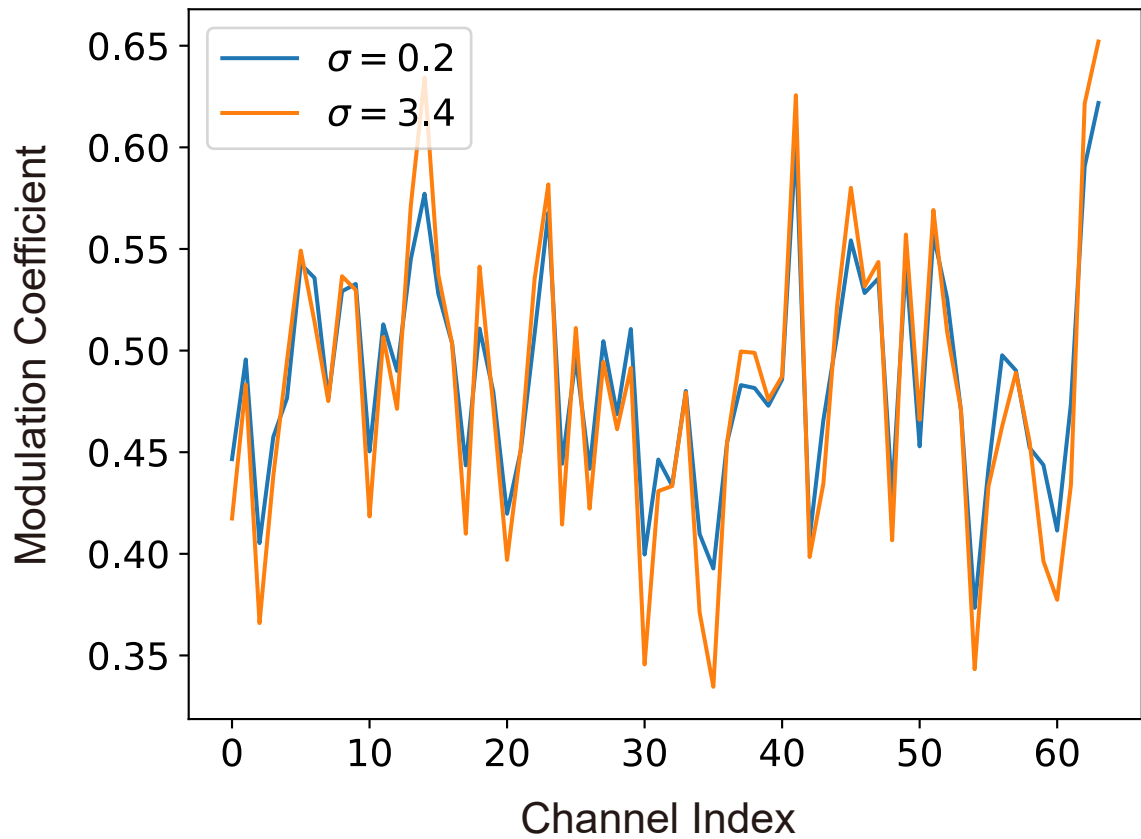

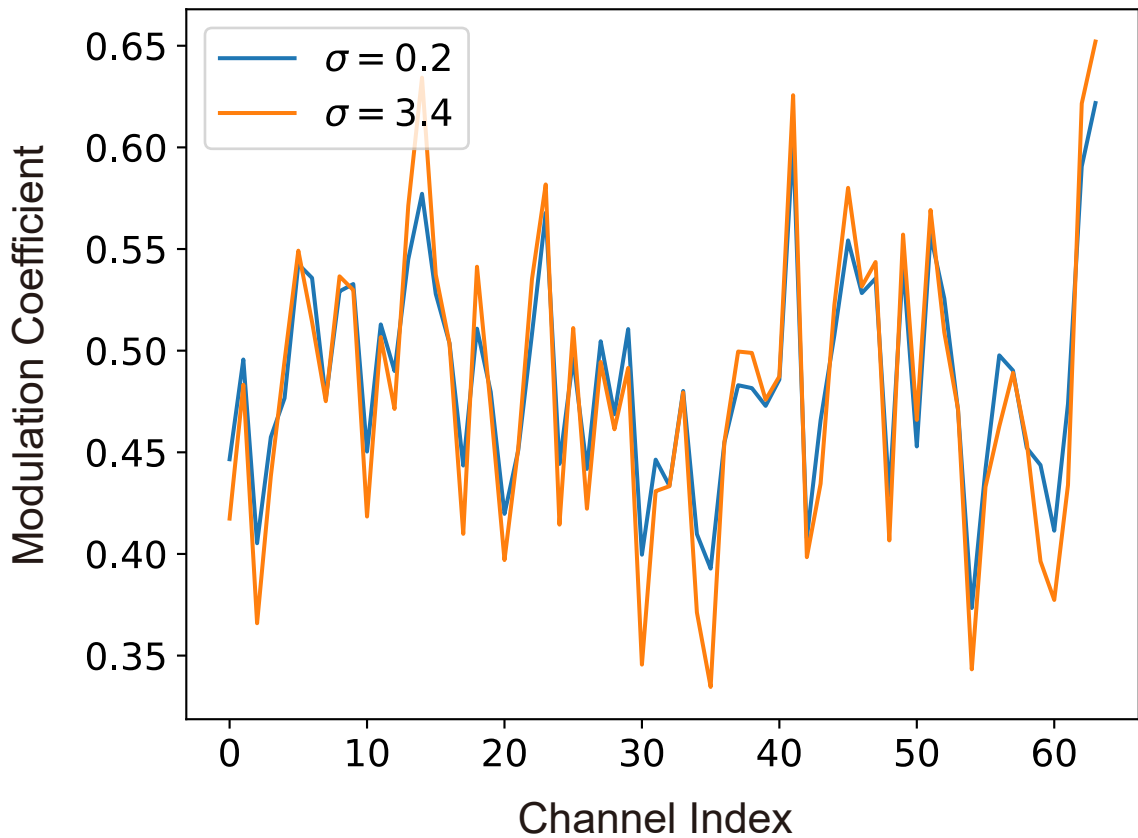

Supplement: Supplementary file 1 [file supp_fig5.pdf]
